# Supplementary material for: A Paradigm For Collaborative Pervasive Fog Computing Ecosystems at the Network Edge
Source: arXiv:2404.09354 source file (2024-04-17)
Supplement: Supplementary file 1 [file appendix.tex]

This appendix details the game theory approach adopted for the f2f2 cooperation. We motivate the use of cooperation probabilities coupled with cooperation fairness. Cooperation is best understood and analyzed when casted as a {\em Game}. Suppose that each node is an agent with only two pure strategies: either to {\em defeat}, strategy 0, or to {\em cooperate}, strategy 1. Note that at this stage we do not consider a cooperation probability. The payoff of this game is the reduction in the fraction of tasks not sent to the cloud. Due to the random arrivals of tasks, this payoff cannot be measured per-task basis. Since this payoff is an average, we will assume that a strategy is played for an amount of time, called a round, long enough to make this estimation reliable, and allowing nodes to coordinate the change of their corresponding strategies at the beginning of a new round.

\begin{table}
 \centering
    \begin{tabular}{*{4}{c|}}
      \multicolumn{2}{c}{} & \multicolumn{2}{c}{Node $n_2$}\\\cline{3-4}
      \multicolumn{1}{c}{} &  & 0  & 1\\\cline{2-4}
      \multirow{2}*{Node $n_1$}  & 0 & 52,52 & 71,43 \\\cline{2-4}
      & 1 & 43,71 & 63,63 \\\cline{2-4}
    \end{tabular}
      \caption{A numerical example of the payoff matrix. The payoff of node $n_2$ is the left value of any entry of the table.}
  \label{tab:Payoff2a} 
\end{table}

Table~\ref{tab:Payoff2a} measures the payoff matrix of this game, where the payoff of node $n_i$ is $1-b_i$, $b_i$ being the blocking probability of the $MC$ model for $\lambda_1=\lambda_2=0.95$. We can see that 00 is a Nash equilibrium. In fact, suppose the game is played sequentially and starts from $(00)$. If node $n_1$ changes its strategy to 1, its utility decreases while the utility of node  $n_2$ increases. Node $n_2$ best strategy is to {\em defeat} to avoid reducing its utility. But if node $n_2$ decides to not cooperate, node $n_1$ changes its strategy back to 0 which increases its utility.

One can argue that this deadlock condition can be avoided by making a node having a memory and allowing the game to be repeated: if node $n_2$ observes that if it will not change its strategy, node $n_1$ will return back to not cooperate, the next time node $n_1$ will change the strategy from 0 to 1, and node $n_2$ will also change its strategy from 0 to 1, which corresponds to a payoff of $(11)$ which is higher than the payoff of $(00)$. As node $n_1$ will now see its utility increasing, it will not fall back to the no cooperating strategy. 

%Note that a node can detect the strategy used by the other node by measuring the utility during a round.

In a real system however, it may happen that even if a node {\it wants} to cooperate it cannot share its server due to overloaded resources. This particular condition makes the cooperation among nodes hard to be reached. As nodes belongs to two different providers, we cannot assume that nodes do not cheat. Indeed, if  nodes trust each other they simply always cooperate.

\begin{table}
 \centering
    \begin{tabular}{*{6}{c|}}
      \multicolumn{2}{c}{} & \multicolumn{3}{c}{Node $n_2$}\\\cline{3-5}
      \multicolumn{1}{c}{} &  & 0  & 0.5 & 1 \\\cline{2-5}
      \multirow{3}*{Node $n_1$}  & 0 & 52,52 & 63,47 & 71,43 \\\cline{2-5}
      & 0.5 & 47,63 & 58,58 & 66,55  \\\cline{2-5}
      & 1 & 43,71 & 55,66 & 63,63  \\\cline{2-5}
    \end{tabular}
      \caption{A numerical example of the payoff matrix for the previous two cooperating nodes, with 3 strategies.}
  \label{tab:Payoff2} 
  \end{table}

We assume now that nodes cheat, say node $n_2$ cheats and does not share its server even when it is idle. Using our model, this behavior can be expressed as node $n_2$ cooperates with probability, say $p_2=0.5$. Node $n_1$ cannot detect the reason why node $n_2$ is not sharing its server. 

Now, assume that the game starts from 00, and node $n_1$ changes its strategy from 0 to 1. Node $n_2$ knows that if it will not cooperate, then node $n_1$ will fall back to strategy 1. However, let see what happens if node $n_2$ cooperates with probability $p_2$. Table~\ref{tab:Payoff2} reports the Payoff matrix of this new Game, where strategy label denotes the cooperating probability. The reaction of node $n_2$ to a change in the node $n_1$ strategy from 0 to 1, can now just be to move from 0 to 0.5 instead of a move from 0 to 1. This induces an increase of the utility of node $n_1$ from 52 to 55 and of node $n_2$ from 52 to 66. Hence node $n_1$ will keep this strategy. Actually, node $n_2$ can theoretically set $p_2$ to the minimal value such that $b_1<b^0_1$ as it makes node $n_1$ confirm its strategy and obtain however a minimal utility.

\begin{figure}[ht] 
\centering
  \includegraphics[width=0.8\linewidth]{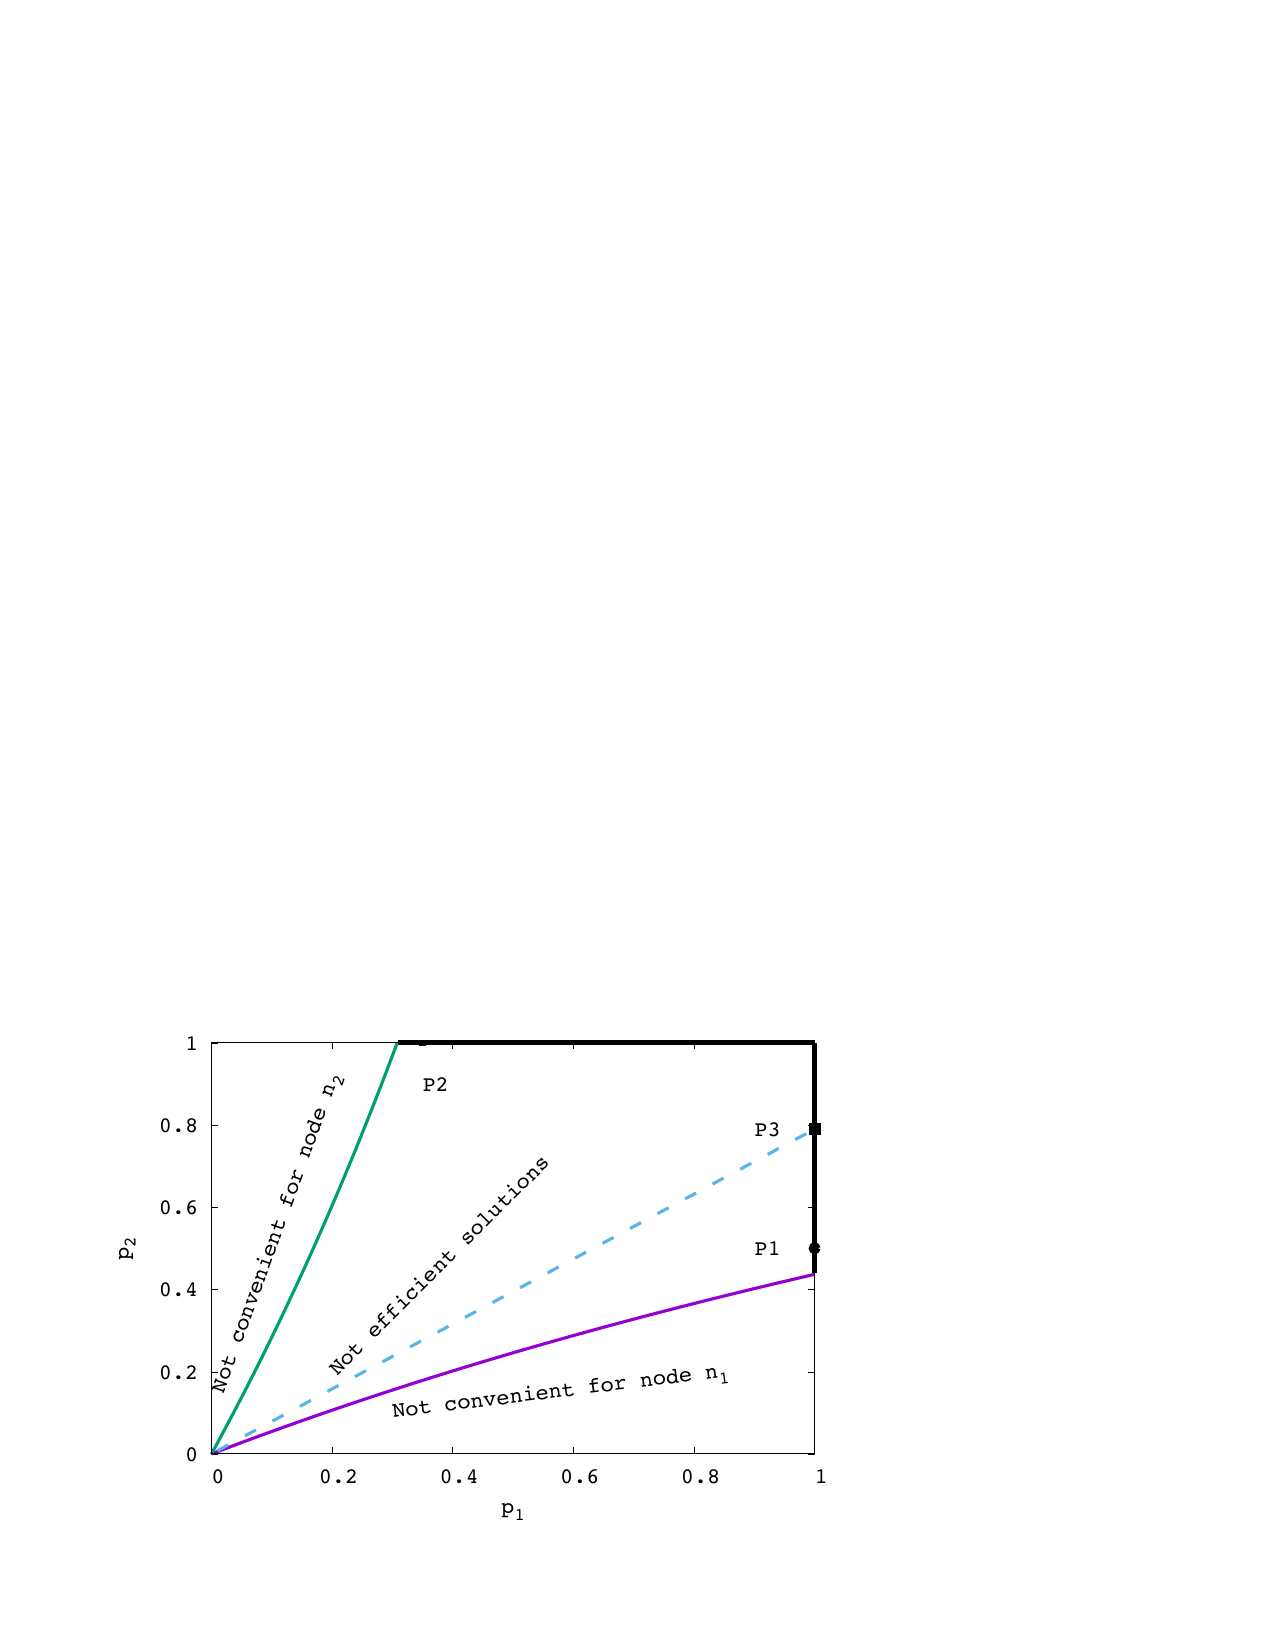}
    \caption{The cooperation probability domain for $\lambda_1=0.95,\lambda_2=0.8$. The three points represent possible stable points for a two node cooperating game. Any point between the two lines provide lower blocking probabilities to both nodes compared to no cooperation. The black line is the  Pareto efficient set. }
    \label{fig:PARETO_09504NEW} 
\end{figure}

Fig.~\ref{fig:PARETO_09504NEW}, uses the $MC$ model with $\lambda_1=0.9, \lambda_2=0.8$, to show the $p_1 \times p_2$ plane with two lines. The bottom line is the contour line $b_1(p_1,p_2)=b^{0}_1$ and the top line is the one of $b_2(p_1,p_2)=b^{0}_2$. Any $p_2$ above the line at the bottom improves node $n_1$'s blocking probability compared to its blocking probability when not cooperating, $b^{0}_1$. Following our previous analysis, the point $P1$ represents a stable pair for the cooperation probabilities when node $n_1$ starts to cooperate and $P2$ the probabilities when node $n_2$ starts to cooperate. 

The main issue with this solution is the fact that while node $n_1$ is undoubtedly gaining compared to when it does not cooperate, the reduction of node $n_2$'s blocking probability is paradoxically (much) higher. node $n_2$ in fact had any interest to initiate to cooperate. This means that the node that starts to cooperate is somehow penalized: If node $n_2$ is the initiator node (\ie starts the cooperation), node $n_1$ registers a higher gain. Note that under the formal point of views all points are Pareto optimal, with the Pareto optimal set being the two vertical and horizontal segments, as discussed in Property~\ref{property1}.

The two nodes can change their cooperation probability at 'smaller' steps, in the hope to reach a better agreement. \eg node $n_1$ can increase its cooperation probability at steps $\delta p_1$ at wait for the reply of node $n_2$. If node $n_2$ replies with increasing its cooperation probability then node $n_1$ could increase its cooperation probability to $2 \delta p_1$ and so on. Its easy to see that the best reply for node $n_2$ is to increase its cooperation probability at steps $\delta p_2$ just enough to get $b_1(\delta p1,\delta p_2) <b^{0}_1$, so that eventually the point (close to) $P1$ is reached (In the Figure \ref{fig:PARETO_09504NEW} this could be visualized as a zig-zag line starting from (0,0) and landing close to point $P1$.)

We argue that this analysis may discourage a node to initiate to cooperate and can provide a deadlock condition as well. For this reason, we guess that some additional and measurable condition that the two nodes may agree upon, may lead to a better way to cooperate. For this reason we have introduced the notion of fairness. Point $P3$ in the Figure show the fair cooperation point according to our definition.
